# Supplementary material for: Beyond VQA: Generating Multi-word Answer and Rationale to Visual Questions
Source: arXiv:2010.12852 source file (2021-06-17)
Supplement: Supplementary file 2 [file 1_high_level_architecture.tex]

\section{High-level conceptual illustration of model}
For a better understanding of our approach, Figure~\ref{fig:proposed_architecture_alternate} presents a high-level illustration of our proposed generation refinement model. Let $A_1=(a_{11},a_{12},...,a_{1l_a})$, $R_1=(r_{11},r_{12},...,r_{1l_r})$, $A_2=(a_{21},a_{22},...,a_{2l_a})$ and $R_2=(r_{21}\\,r_{22},...,r_{2l_r})$ be the generated answer, generated rationale, refined answer and refined rationale sequences respectively, where $a_{ij}$ and ${r_{ij}}$ are discrete random variables taking values from common vocabulary $\mathcal{V}$. $F$ is a random variable that indicates the common input to every module.
 \begin{figure}[H]
    % %\vspace{-2pt}
    \centering
    \includegraphics[width=0.9\columnwidth]{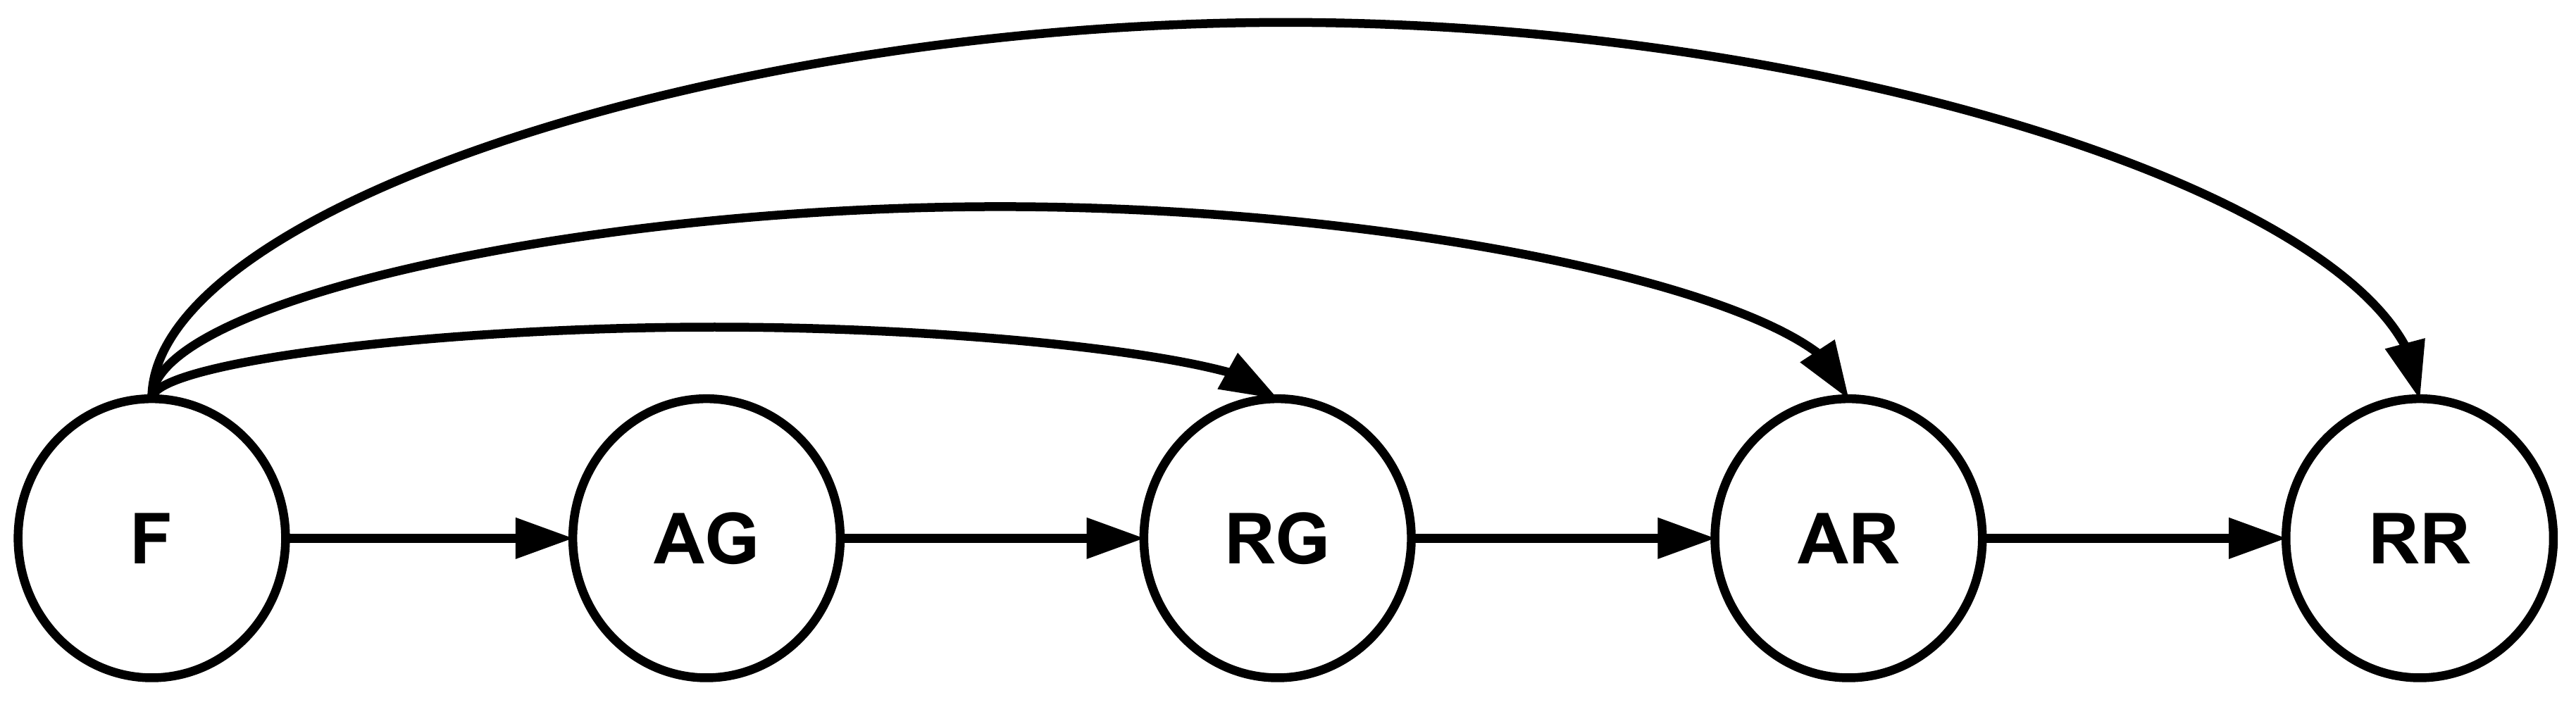}
    %  %\vspace{-16pt}
    \caption{High-level illustration of our proposed Generation-Refinement model.}
    %\vspace{-12pt}
      \label{fig:proposed_architecture_alternate}
\end{figure}

The objective now is to maximize the likelihood $P(A_1,R_1,A_2,R_2 | F)$ given by:
%\vspace{-3pt}
\begin{align}
P(A_1, R_1, A_2, R_2 | F)&=P(A_1, R1 | F) P(A_2, R_2 | F, A_1, R_1) \nonumber\\
&=P(A_1|F)P(R_1|F,A_1)\nonumber\\& {}P(A_2|F,A_1,R_1)P(R_2 | F, A_1, R_1, A_2)\label{eqn:14}
% P(A_1, R_1, A_2, R_2 | F)&=P(A_1, R1 | F) P(A_2, R_2 | F, A_1, R_1) \nonumber\\
% &=P(A_1|F)P(R_1|F,A_1)P(A_2|F,A_1,R_1)P(R_2 | F, A_1, R_1, A_2)\label{eqn:14}
%\vspace{-5pt}
\end{align}
Each term in the RHS of Equation~\ref{eqn:14} can be computed by a distinct LSTM. Minimizing the sum of losses of the four LSTMs is equivalent to maximizing the joint probability.
The overall loss is the sum of four cross-entropy losses, one for each LSTM, given below:
%\vspace{-9pt}
\begin{equation}
    \mathcal{L} = - \bigg( \sum_{t=1}^{l_a} \log p^{\theta_1}_t + \sum_{t=1}^{l_r} \log p^{\theta_2}_t + \sum_{t=1}^{l_a} \log p^{\theta_3}_t + \sum_{t=1}^{l_r} \log p^{\theta_4}_t\bigg)
\end{equation}
\noindent where $\theta_i$ represents the $i^{th}$ sub-module LSTM, $p_t$ is the conditional probability of the $t^{th}$ word in the input sequence as calculated by the corresponding LSTM, $l_a$ indicates the ground-truth answer length, and $l_r$ the ground truth rationale length.
