# Supplementary material for: Beyond VQA: Generating Multi-word Answer and Rationale to Visual Questions
Source: arXiv:2010.12852 source file (2021-06-17)
Supplement: Supplementary file 5 [file 7_Visual_atten_maps.tex]

%\vspace{-4pt}
\section{How interpretable are a results? A Study using attention maps}
%\vspace{-4pt}
We visualized the attention weights for the model with and without the Refinement module. Addition of a Refinement module causes the model to attend to more relevant regions and leads to better answers and rationales.
Figure ~\ref{fig:attention maps2} 
presents an example to illustrate the visualization of the attention weights used by generation model and generation-refinement model while generating each word of answer and rationale. The attention map visualizations also show that a model is visualizing the appropriate entities in the given image when generating the answer and rationale.

\begin{figure*}
\centering
    \subfloat{\includegraphics[width=\linewidth]{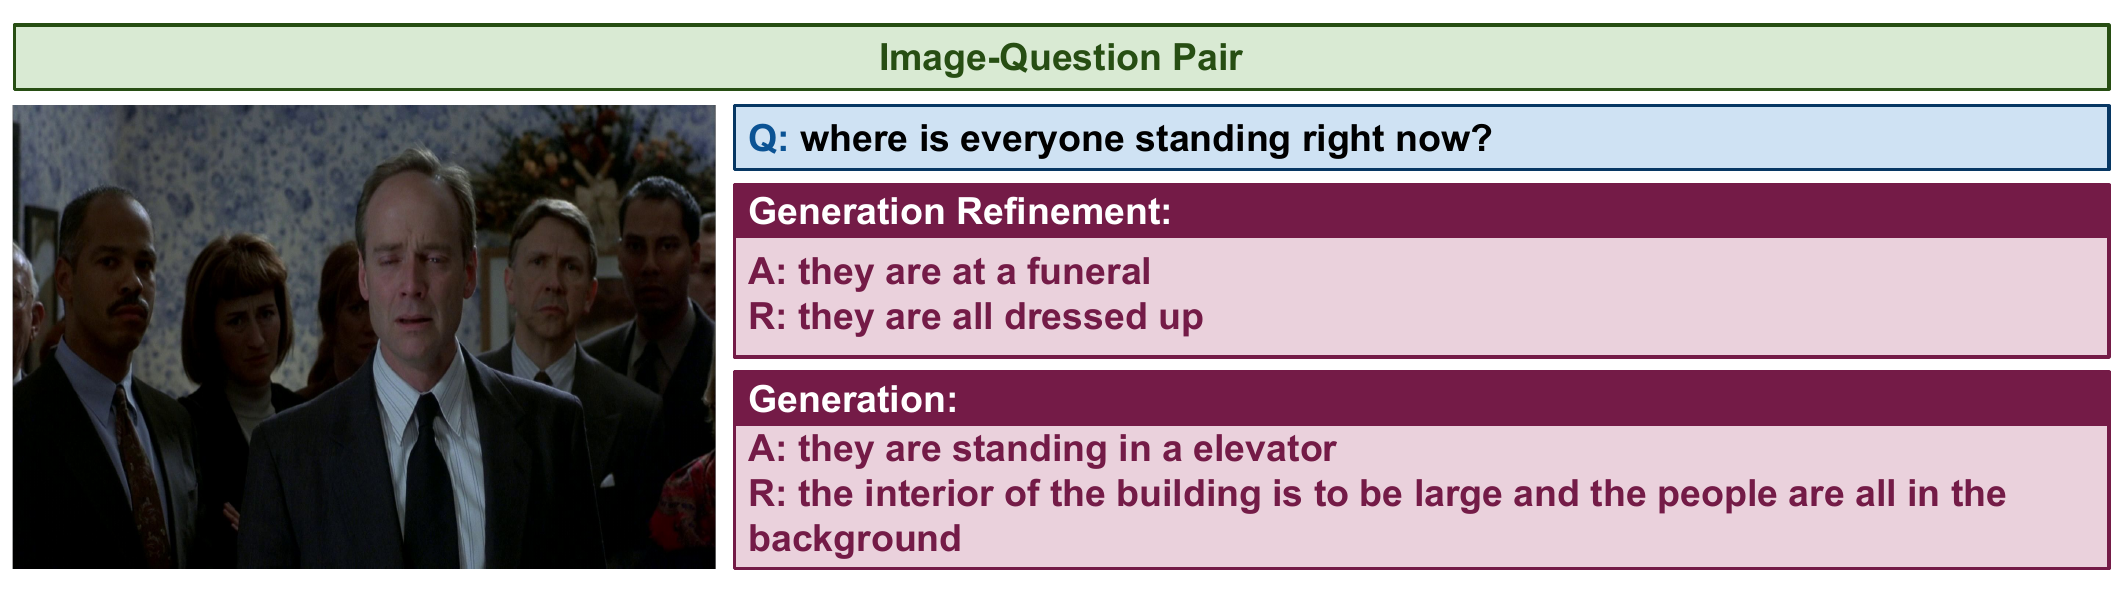}\label{fig:q1}}\\[-2ex]
    \subfloat{\includegraphics[width=\linewidth]{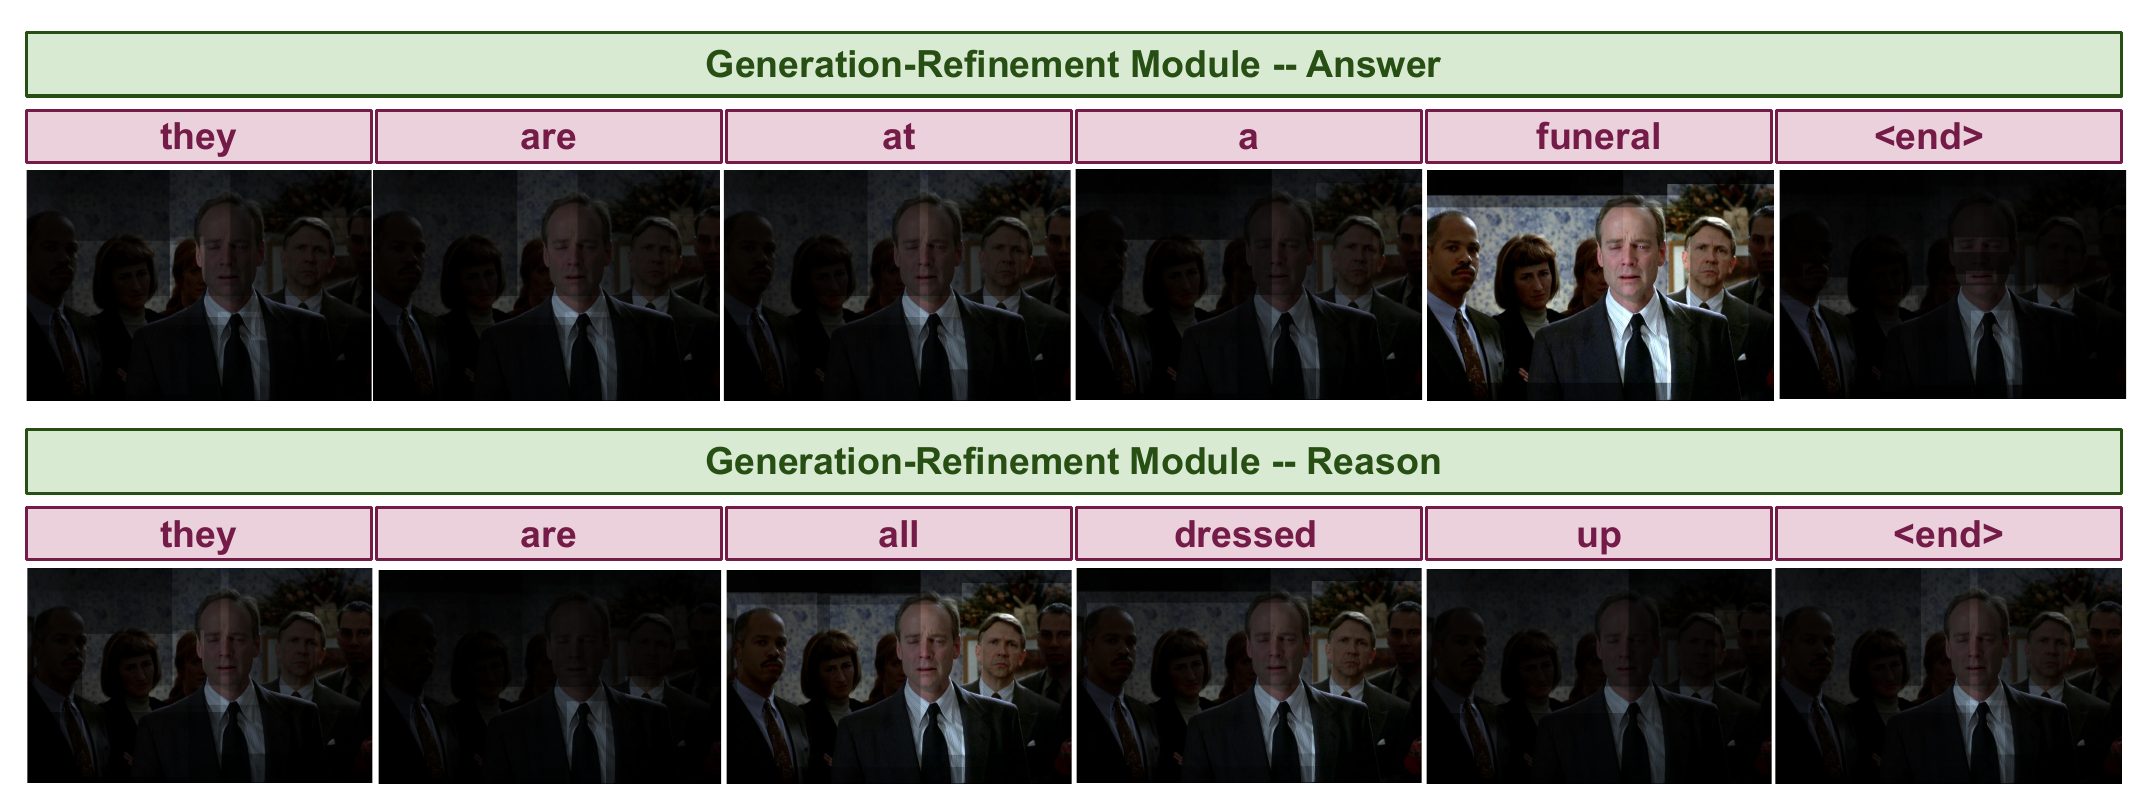}\label{fig:q2}}\\[-2ex]
    \subfloat{\includegraphics[width=\linewidth]{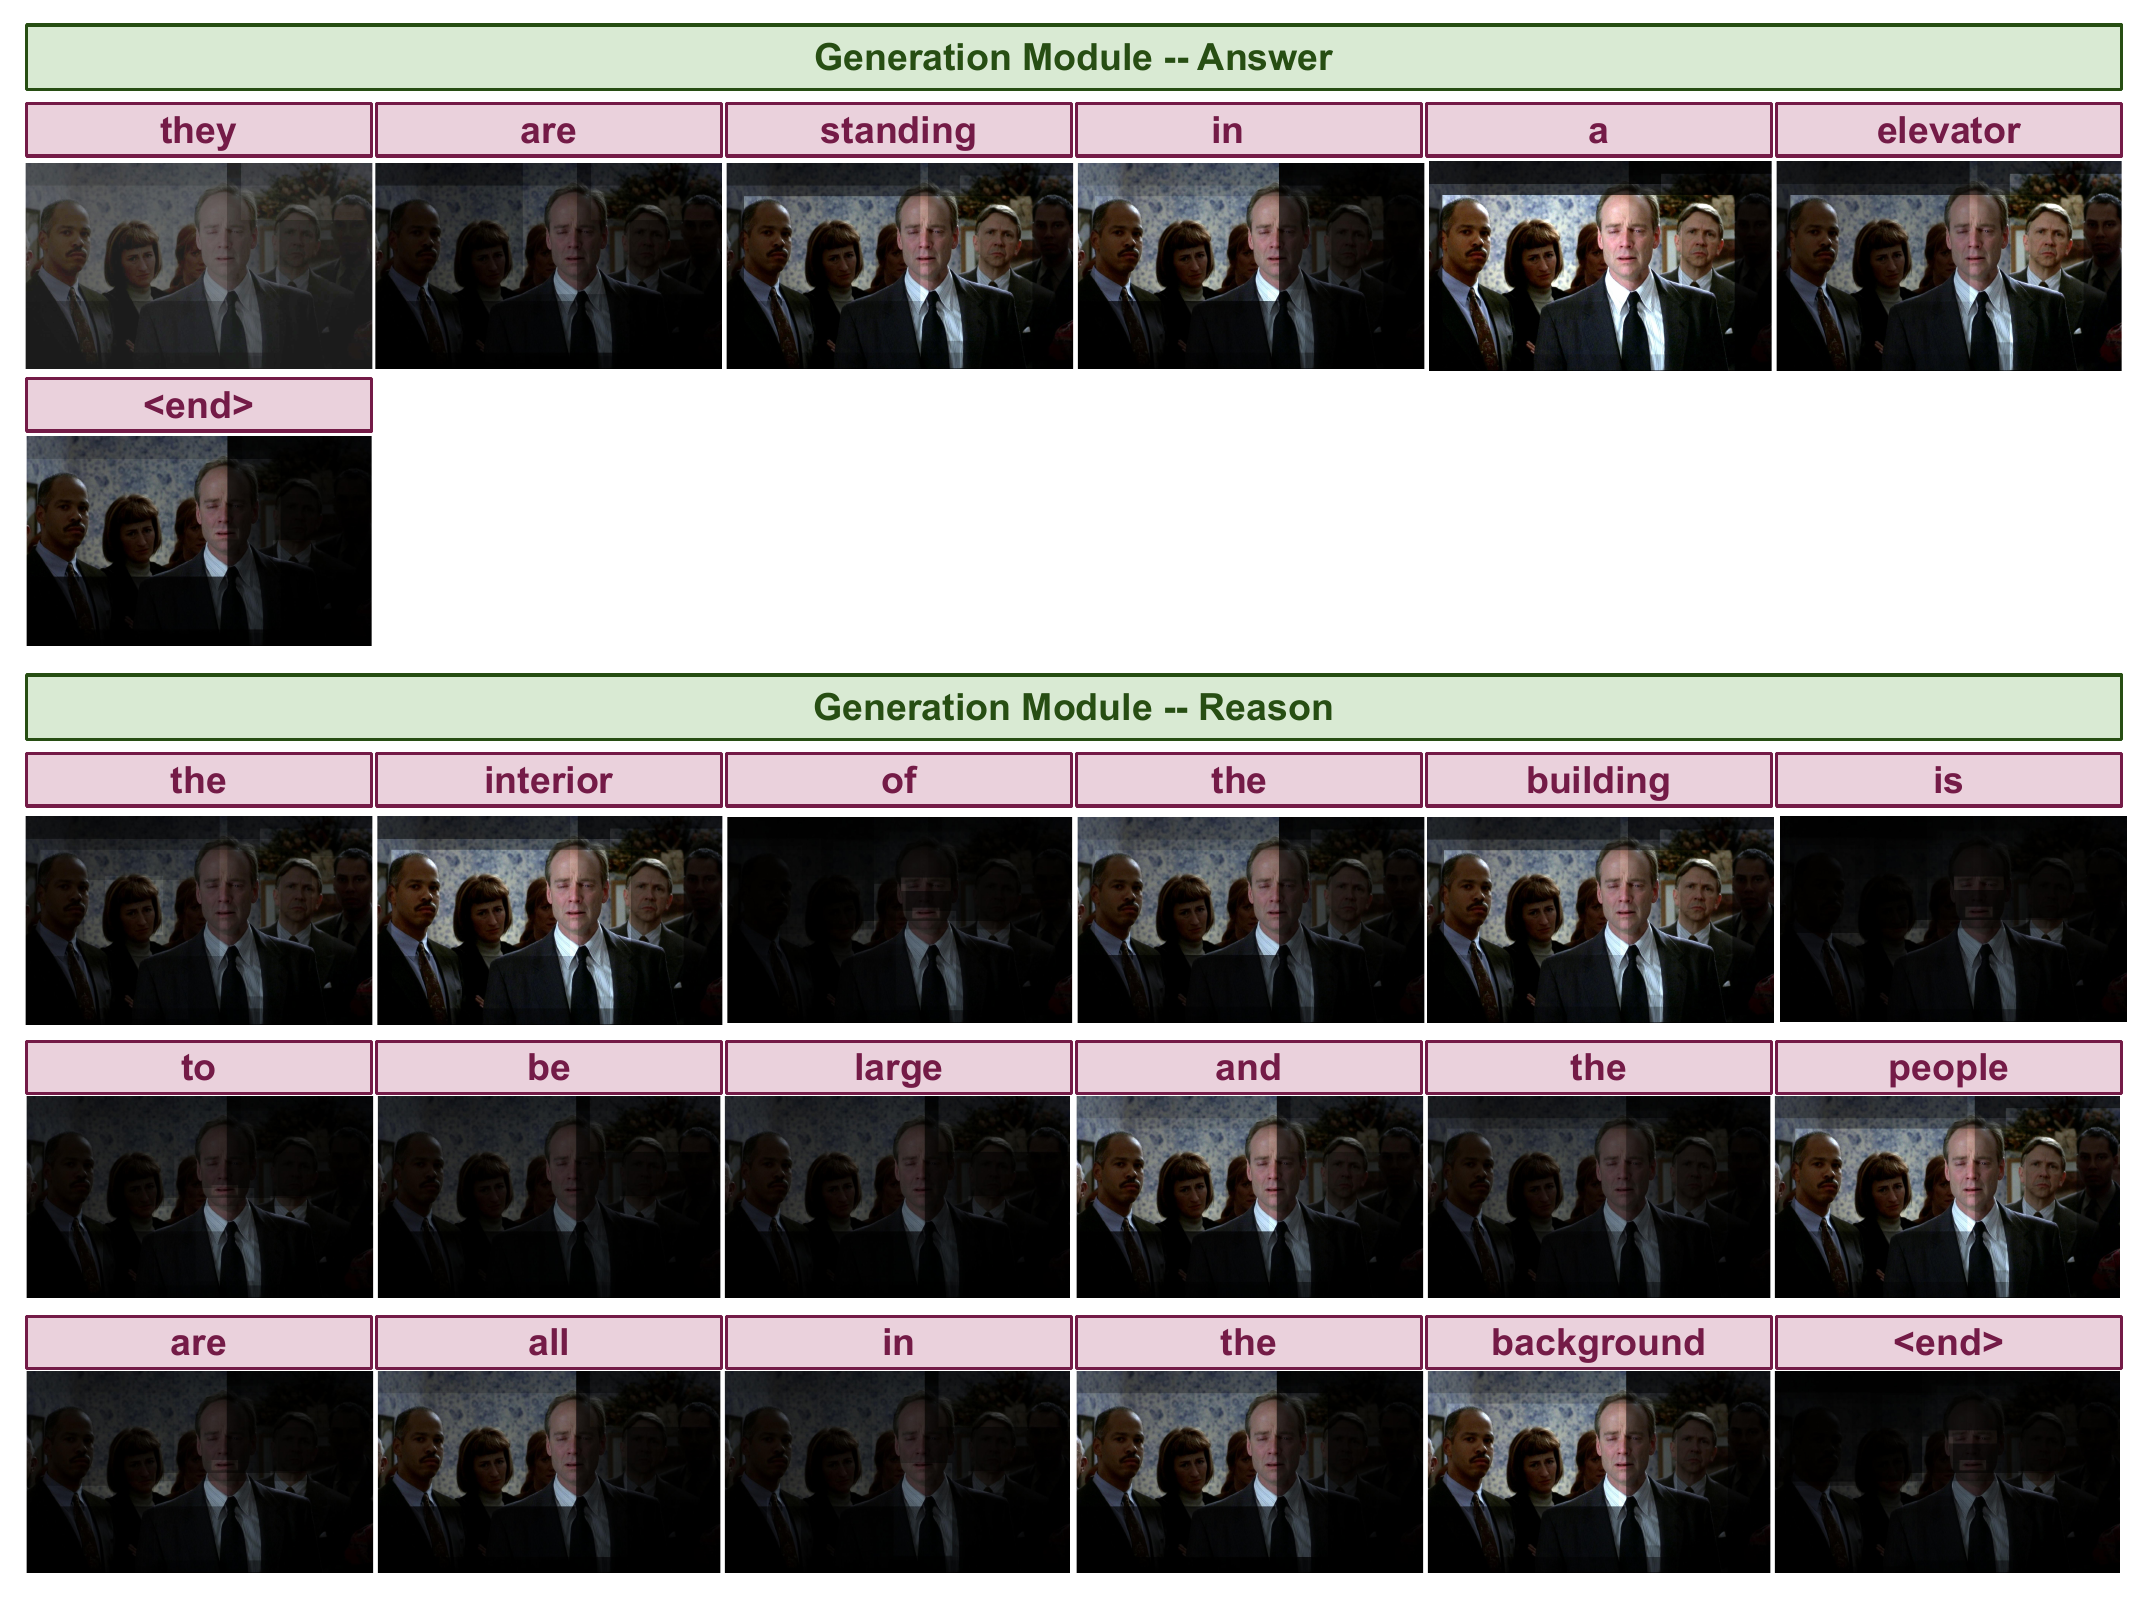}\label{fig:q3}}
\caption{\textit{(Best viewed in color)} Visualization of attention weights that models use while generating each word.}
\label{fig:attention maps2}
\end{figure*}
